# Supplementary material for: Nonlinear cavity feeding and unconventional photon statistics in solid-state cavity QED revealed by many-level real-time path-integral calculations
Source: arXiv:1704.03347 source file (2017-09-04)
Supplement: Supplementary file 1 [file supplement.pdf]

# Supplement: Nonlinear cavity feeding and unconventional photon statistics in solid-state cavity QED revealed by many-level real-time path-integral calculations

M. Cygorek,[1] A. M. Barth,[1] F. Ungar,[1] A. Vagov,[1] and V. M. Axt[1]
[1] *Theoretische Physik III, Universität Bayreuth, 95440 Bayreuth, Germany*

## REFORMULATON OF THE ITERATIVE REAL-TIME PATH-INTEGRAL ALGORITHM

In this section, we describe in detail the iterative real-time path-integral algorithm used in the main text for the description of solid-state cavity QED systems. Our starting point is a well established iteration scheme for the so called *augmented density matrix* that has been introduced and implemented before [1–4] to perform the sum over paths needed to obtain the reduced density matrix. First, in the next subsection we shall summarize the main results of this scheme in order to have a basis for the reformulation of the algorithm as an iteration scheme for a partially summed augmented density matrix. This reformulation is the key for the huge reduction of the numerical effort which enabled us to perform a numerically complete study for a system with 41 fully coupled levels interacting with a continuum of acoustic phonons. As this reformulation is not restricted to the specific system considered in the main text, we shall formulate the algorithm for a general $N$-level system that can be subdivided into $N_g$ groups with identical pure-dephasing-type couplings to a continuum of bosons within each group and explain alongside how the general scheme reduces to the special case treated in the main text.

### Augmented density matrix iteration for simulating the system dynamics

The time evolution of the full many-body statistical operator $\hat\rho$ for a system with $N$ levels coupled to a continuum of independent boson oscillators is given by:

$$\frac{\partial}{\partial t}\hat\rho = \mathcal{L}_N[\hat\rho] + \mathcal{L}_{\rm osc}[\hat\rho], \tag{1}$$

where $\mathcal{L}_N$ is the Liouville operator for the evolution of the $N$-level system in the absence of the boson oscillators. It can usually be decomposed according to:

$$\mathcal{L}_N[\hat\rho] = \frac{1}{i\hbar}\{\hat H_N, \hat\rho\}_- + \mathcal{L}_{\rm loss}[\hat\rho], \tag{2}$$

where $\{,\}_-$ is the commutator and $\hat H_N$ stands for an $N$-level Hamiltonian, which besides defining couplings between the $N$ levels may contain a time dependent driving. Let $\{|\mu\rangle\}$ be a basis of ket states for the $N$-level system and $\{\langle\nu|\}$ the corresponding bra states. Then, $\hat H_N$ can be written as:

$$\hat H_N = \sum_{\mu\nu} H^N_{\mu\nu}(t)\,|\mu\rangle\langle\nu|. \tag{3}$$

In the specific case studied in the main text, the basis $|\nu\rangle$ comprises the states $|G, n_x\rangle$, $|X, n_x-1\rangle$ with $1\le n_x\le 20$ as well as $|G,0\rangle$ and $H^N_{\mu\nu}(t)$ is obtained by taking the corresponding matrix elements of Eq. (1) in the main text, i.e. $\hat H_N$ comprises here the Jaynes-Cummings-type couplings between the basis states as well as the dipole coupling of the dot to an external laser field.

$\mathcal{L}_{\rm loss}$ describes non-Hamiltonian contributions to the dynamics which arise in open quantum systems primarily by losses due to the coupling with the surrounding environment. Often such contributions can be represented by Liouville operators in the so called Lindblad form: [5]

$$\mathcal{L}_{\rm loss} = \sum_p \kappa_p\big[\hat A_p\hat\rho\hat A_p^\dagger - \frac{1}{2}\{\hat\rho, \hat A_p^\dagger\hat A_p\}_+\big], \tag{4}$$

where $\{,\}_+$ denotes the anti-commutator, $\hat A_p$ are system operators characterizing the process to be modeled and $\kappa_p$ are the corresponding rates. This form applies in particular to the cavity losses considered in the main text. Finally

$$\mathcal{L}_{\rm osc}[\hat\rho] = \frac{1}{i\hbar}\{\hat H_{\rm osc}, \hat\rho\}_-, \quad \text{with} \quad \hat H_{\rm osc} = \hbar\sum_{\mathbf q}\omega_{\mathbf q}\hat b^\dagger_{\mathbf q}\hat b_{\mathbf q} + \hbar\sum_{\nu\mathbf q}\big(\gamma^\nu_{\mathbf q}\hat b^\dagger_{\mathbf q} + \gamma^{\nu *}_{\mathbf q}\hat b_{\mathbf q}\big)|\nu\rangle\langle\nu| \tag{5}$$

is the Liouville operator accounting for a pure-dephasing type interaction with bosonic oscillators. $\hat{b}^\dagger_{\mathbf{q}}$ and $\hat{b}_{\mathbf{q}}$ are, respectively, the creation and annihilation operators of bosons in mode $\mathbf{q}$ with energy $\hbar\omega_{\mathbf{q}}$ while $\gamma^\nu_{\mathbf{q}}$ defines the coupling strength between the mode $\mathbf{q}$ and the state $|\nu\rangle$.

We are interested in the dynamics of the reduced density matrix $\bar{\rho}$ which is obtained from the statistical operator of the total system by tracing over the oscillator degrees of freedom and taking matrix elements in the basis of the $N$-level system: $\bar{\rho}_{\nu\mu} = \langle\nu|\mathrm{Tr}_{\rm osc}\big(\hat{\rho}\big)|\mu\rangle$. It is known for a long time that $\bar{\rho}_{\nu\mu}$ can be represented as a sum over paths when the system dynamics is Hamiltonian [1]. Recently, it has been shown that this still holds when in addition to Hamiltonian contributions the Liouville operator for the $N$-level system of interest also contains non-Hamiltonian parts [4]. As in the latter paper, we consider an equally spaced discretization of time $t_\ell = \Delta t\,\ell$ with time steps of width $\Delta t$ and integer $\ell$ and label the states of the $N$-level system at time $t_\ell$ by $\nu_\ell$ or $\mu_\ell$. Furthermore, we assume that at time $t_0$ the system is in its ground state $|0\rangle$ while the oscillators are in a thermal distribution at temperature $T$. Then the sum-over-paths representation of the reduced density matrix is given by [4]:

$$\bar{\rho}_{\nu_n\mu_n} = \sum_{\substack{\nu_0\cdots\nu_{n-1}\\ \mu_0\cdots\mu_{n-1}}} R^{\mu_n\cdots\mu_0}_{\nu_n\cdots\nu_0}, \qquad \text{with} \qquad R^{\mu_n\cdots\mu_0}_{\nu_n\cdots\nu_0} := \bar{\rho}_{\nu_0\mu_0}\prod_{\ell=1}^{n}\mathcal{M}^{\nu_{\ell-1}\mu_{\ell-1}}_{\nu_\ell\mu_\ell}\exp\Big(\sum_{\ell=1}^{n}\sum_{\ell'=1}^{\ell}S^{\nu_{\ell'}\mu_{\ell'}}_{\nu_\ell\mu_\ell}\Big). \tag{6}$$

Here, a path is any possible sequence $\nu_0\ldots\nu_{n-1}$ of states that the system may run through while stepping forward in time from $t_0$ to $t_{n-1}$. Equation (6) involves two summations over all paths since for obtaining the reduced density matrix the ket- $|\mu\rangle$ as well as the bra-states $\langle\nu|$ have to be propagated. Thus, for an $N$-level system the sum runs over $N^{2n}$ terms. Each term contains three factors: the initial reduced density matrix $\bar{\rho}_{\nu_0\mu_0}$ at time $t_0$, a factor $\prod_{\ell=1}^{n}\mathcal{M}^{\nu_{\ell-1}\mu_{\ell-1}}_{\nu_\ell\mu_\ell}$ accounting for the dynamics induced by $\mathcal{L}_N$ and a factor $\exp\big(\sum_{\ell=1}^{n}\sum_{\ell'=1}^{\ell}S^{\nu_{\ell'}\mu_{\ell'}}_{\nu_\ell\mu_\ell}\big)$ capturing the influences of the oscillators.

$\bar{\rho}_{\nu_0\mu_0}$ is determined by the initial conditions to be the reduced density matrix of the system ground state. The factor $\prod_{\ell=1}^{n}\mathcal{M}^{\nu_{\ell-1}\mu_{\ell-1}}_{\nu_\ell\mu_\ell}$ is most easily defined by introducing the time evolution operator $\mathcal{M}_{t,t'}$ for the propagation of the $N$-level system without oscillator coupling from time $t$ to $t'$:

$$\mathcal{M}_{t,t'}[\cdot] = \mathcal{T}\exp\bigg(\int_t^{t'}\mathcal{L}_N dt'\bigg)\big[\,\cdot\,\big], \tag{7}$$

i.e., $\mathcal{M}_{t,t'}$ maps the reduced density matrix at time $t$ to its values reached at time $t'$ when the system evolves under the action of the Liouville operator $\mathcal{L}_N$. For time-independent $\mathcal{L}_N$, $\mathcal{M}_{t,t'}$ can be conveniently constructed using standard methods for taking the exponential of a finite size matrix. Alternatively, one can solve numerically the equation of motion for the reduced density matrix in the oscillator-free case (i.e., solving an ordinary differential equation for a $N\times N$ matrix). The factors $\mathcal{M}^{\nu_{\ell-1}\mu_{\ell-1}}_{\nu_\ell\mu_\ell}$ are then obtained by acting with $\mathcal{M}_{t_{\ell-1},t_\ell}$ on the basis projectors $|\nu_{\ell-1}\rangle\langle\mu_{\ell-1}|$ and taking the matrix elements between states $|\nu_\ell\rangle$ and $|\mu_\ell\rangle$ of the result:

$$\mathcal{M}^{\nu_{\ell-1}\mu_{\ell-1}}_{\nu_\ell\mu_\ell} = \langle\nu_\ell|\,\mathcal{M}_{t_{\ell-1},t_\ell}\big[\,|\nu_{\ell-1}\rangle\langle\mu_{\ell-1}|\,\big]\,|\mu_\ell\rangle. \tag{8}$$

Finally, the oscillator influence is encoded in the functions $S^{\nu_{\ell'}\mu_{\ell'}}_{\nu_\ell\mu_\ell}$ which represent a phonon-induced memory with a memory depth $t_\ell - t_{\ell'}$. The explicit expression for $S^{\nu_{\ell'}\mu_{\ell'}}_{\nu_\ell\mu_\ell}$ used for the simulations in the main text are given below. For the discussion of the numerical algorithm only two properties are important: (i) $S^{\nu_{\ell'}\mu_{\ell'}}_{\nu_\ell\mu_\ell}$ depends on the indices $\nu_\ell,\mu_\ell,\nu_{\ell'},\mu_{\ell'}$ only via its dependence on the corresponding couplings $\gamma^{\nu_\ell}_q,\gamma^{\mu_\ell}_q,\gamma^{\nu_{\ell'}}_q,\gamma^{\mu_{\ell'}}_q$ and (ii) for a continuum of oscillators, $S^{\nu_{\ell'}\mu_{\ell'}}_{\nu_\ell\mu_\ell}$ is negligibly small when $t_\ell - t_{\ell'}$ exceeds a certain finite memory time $t_m = n_m\Delta t$.

From the definition of the terms $R^{\mu_n\cdots\mu_0}_{\nu_n\cdots\nu_0}$ one obtains immediately the recurrence:

$$R^{\mu_n\cdots\mu_0}_{\nu_n\cdots\nu_0} = \mathcal{M}^{\nu_{n-1}\mu_{n-1}}_{\nu_n\mu_n}\exp\bigg(\sum_{\ell=1}^{n}S^{\nu_\ell\mu_\ell}_{\nu_n\mu_n}\bigg)R^{\mu_{n-1}\cdots\mu_0}_{\nu_{n-1}\cdots\nu_0}, \qquad n\geq 1 \tag{9}$$

with the initial condition $R^{\mu_0}_{\nu_0} = \bar{\rho}_{\nu_0\mu_0}$. For obtaining an efficient numerical algorithm, in the pioneering work of Makri *et al.* [1, 2] the *augmented density matrix* (ADM) is introduced for $n > n_m$ as $\rho^{\mu_n\cdots\mu_{n-n_m+1}}_{\nu_n\cdots\nu_{n-n_m+1}} := \sum_{\substack{\nu_{n-n_m}\cdots\nu_0\\ \mu_{n-n_m}\cdots\mu_0}} R^{\mu_n\cdots\mu_0}_{\nu_n\cdots\nu_0}$. Exploiting the finite depth of the phonon-induced memory [property (ii)] it was shown in Ref. 1 that the ADM obeys the recursion:

$$\rho^{\mu_n\cdots\mu_{n-n_m+1}}_{\nu_n\cdots\nu_{n-n_m+1}} = \mathcal{M}^{\nu_{n-1}\mu_{n-1}}_{\nu_n\mu_n}\sum_{\substack{\nu_{n-n_m}\\ \mu_{n-n_m}}}\exp\bigg(\sum_{\ell=n-n_m}^{n}S^{\nu_\ell\mu_\ell}_{\nu_n\mu_n}\bigg)\rho^{\mu_{n-1}\cdots\mu_{n-n_m}}_{\nu_{n-1}\cdots\nu_{n-n_m}}. \tag{10}$$

From the ADM, the reduced $N$-level density matrix can be obtained by:

$$\bar{\rho}_{\nu_n\mu_n}(t_n) = \sum_{\substack{\nu_{n-1}\dots\nu_{n-n_m+1}\\ \mu_{n-1}\dots\mu_{n-n_m+1}}} \rho^{\mu_n\dots\mu_{n-n_m+1}}_{\nu_n\dots\nu_{n-n_m+1}}. \quad (11)$$

The main advantage of using the above recurrence for the ADM is that after reaching the memory time $t_m$ the effort for a further propagation step does no longer increase as the number of elements of the ADM stays at $N_{ADM} = N^{2n_m}$. In this way, the iterative scheme allows one to calculate the dynamics up to arbitrary final times $t_n$.

### Decomposition into groups and recurrence for a partially summed augmented density matrix

The central methodological improvement presented in this article is based on the observation that in many situations, some states $\nu$ and $\mu$ of the $N$-level system couple identically to the bath of bosons, i.e. $\gamma_q^\mu = \gamma_q^\nu$. In this case, the numerical complexity of the real-time path-integral method can be drastically decreased as follows:

Decompose the $N$ levels into $N_g$ groups where the states within a single group have the same coupling to the boson modes. Relabel the states $|\nu\rangle \to |\lambda, k\rangle$ and $|\mu\rangle \to |\bar{\lambda}, \bar{k}\rangle$, where $\lambda = \{1, 2, \dots, N_g\}$ denotes the group and $k$ distinguishes the different states within the respective group. As a result, the coupling can be described by the group index $\gamma_q^\lambda := \gamma_q^{(\lambda,k)}$, $\forall k$. Since the phonon-memory functions $S^{\nu_{\ell'}\mu_{\ell'}}_{\nu_\ell\mu_\ell}$ depend on the state indices only via their dependence on the phonon couplings [property (i)], the influence functional in Eq. (10) can be written as:

$$\sum_{\ell=n-n_m}^{n} S^{\nu_\ell\mu_\ell}_{\nu_n\mu_n} = \sum_{\ell=n-n_m}^{n} S^{(\lambda_\ell,k_\ell)(\bar{\lambda}_\ell,\bar{k}_\ell)}_{(\lambda_n,k_n)(\bar{\lambda}_n,\bar{k}_n)} = \sum_{\ell=n-n_m}^{n} S^{\lambda_\ell\bar{\lambda}_\ell}_{\lambda_n\bar{\lambda}_n} =: S^{\bar{\lambda}_n\dots\bar{\lambda}_{n-n_m}}_{\lambda_n\dots\lambda_{n-n_m}}. \quad (12)$$

Because the influence functional no longer depends on the index $k$ of levels within a group, it is possible to obtain the reduced $N$-level density matrix $\bar{\rho}_{\nu_n\mu_n}(t_n)$ from a partially summed ADM defined as:

$$\rho^{(\bar{\lambda}_n,\bar{k}_n)\bar{\lambda}_{n-1}\dots\bar{\lambda}_{n-n_m+1}}_{(\lambda_n,k_n)\lambda_{n-1}\dots\lambda_{n-n_m+1}} := \sum_{\substack{k_{n-1}\dots k_{n-n_m+1}\\ \bar{k}_{n-1}\dots\bar{k}_{n-n_m+1}}} \rho^{(\bar{\lambda}_n,\bar{k}_n)(\bar{\lambda}_{n-1},\bar{k}_{n-1})\dots(\bar{\lambda}_{n-n_m+1},\bar{k}_{n-n_m+1})}_{(\lambda_n,k_n)(\lambda_{n-1},k_{n-1})\dots(\lambda_{n-n_m+1},k_{n-n_m+1})}. \quad (13)$$

From Eq. (10), one obtains the recursion relation for the partially summed ADM:

$$\rho^{(\bar{\lambda}_n,\bar{k}_n)\bar{\lambda}_{n-1}\dots\bar{\lambda}_{n-n_m+1}}_{(\lambda_n,k_n)\lambda_{n-1}\dots\lambda_{n-n_m+1}} = \sum_{\substack{k_{n-1}\\ \bar{k}_{n-1}}} \mathcal{M}^{(\lambda_{n-1},k_{n-1})(\bar{\lambda}_{n-1},\bar{k}_{n-1})}_{(\lambda_n,k_n)(\bar{\lambda}_n,\bar{k}_n)} \sum_{\substack{\lambda_{n-n_m}\\ \lambda'_{n-n_m}}} \exp\left(S^{\bar{\lambda}_n\dots\bar{\lambda}_{n-n_m}}_{\lambda_n\dots\lambda_{n-n_m}}\right) \rho^{(\bar{\lambda}_{n-1},\bar{k}_{n-1})\bar{\lambda}_{n-2}\dots\bar{\lambda}_{n-n_m}}_{(\lambda_{n-1},k_{n-1})\lambda_{n-2}\dots\lambda_{n-n_m}}. \quad (14)$$

Equation (14) is the central methodological result of this article as it allows the reduction of the number of terms to be iterated from $N_{ADM} = N^{2n_m}$ for the full ADM to $N_{PSADM} = N^2 \cdot N_g^{2(n_m-1)}$ for the partially summed ADM without introducing any approximation.

The above described algorithm has two sources of numerical errors: a discretization error introduced by using a finite time step $\Delta t$ and an error due to the truncation of the memory to $t_m$. We call a simulation *numerically complete* if neither a further reduction of $\Delta t$ nor a further increase of $t_m$ leads to noticeable changes of the resulting reduced density matrix. The required memory time $t_m$ can be easily determined before starting the iteration since the memory functions $S^{\nu_{\ell'}\mu_{\ell'}}_{\nu_\ell\mu_\ell}$ can be evaluated beforehand (see next subsection). For the memory induced by LA phonons $t_m$ is of the order of a few pico seconds. For the system studied in the main text we obtained numerically complete results for $\Delta t = 0.5$ ps and $n_m = 7$. Calculations iterating the full ADM with $n_m = 7$ have been performed for 4-level systems [6, 7] where $N_{ADM} \simeq 2.7 \cdot 10^8$, which is large but manageable. A 5-level system would require $N_{ADM} \simeq 6.1 \cdot 10^9$ which is already ambitious. A system with $N = 41$ and $N_{ADM} \simeq 3.7 \cdot 10^{22}$ is definitely intractable by iterating the full ADM. The number of terms to be iterated using the partially summer ADM in our case with $n_m = 7$, $N = 41$, and $N_g = 2$ is $N_{PSADM} = 6.8 \cdot 10^6$, i.e., more than 15 orders of magnitude less than for the full ADM.

## LA PHONON COUPLINGS TO DOT-CAVITY SYSTEMS

For GaAs-based systems as studied in the main text, the coupling between electrons (holes) confined in a quantum dot with LA phonons is typically dominated by the deformation potential interaction [8], which can be described by:

$$\gamma_{\mathbf{q}}^{e(h)} = \mathcal{F}_{\mathbf{q}}^{e(h)} \frac{|\mathbf{q}| D_{e(h)}}{\sqrt{2V\rho\hbar\omega_{\mathbf{q}}}}, \quad (15)$$

where the form factor $\mathcal{F}^{e(h)}_{\mathbf{q}}$ is the Fourier transform of the absolute square of the electron (hole) wave function, $D_{e(h)}$ is the electron (hole) deformation potential constant, $V$ is the sample volume, and $\rho$ is the mass density of the bulk material. Thus, the phonon coupling to states $|\nu\rangle = |X, n\rangle$ which are product states of the exciton $|X\rangle$ and cavity-photon number states is given by: $\gamma^X_{\mathbf{q}} = \gamma^e_{\mathbf{q}} - \gamma^h_{\mathbf{q}}$. States $|\nu\rangle = |G, n\rangle$ involving the ground state $|G\rangle$ are not dynamically coupled to phonons since the phonons primarily couple to electrons and holes which are both absent in the ground state and thus $\gamma^\nu_{\mathbf{q}} = 0$ in this case. Assuming a harmonic confinement, the wave functions are Gaussians resulting in real Gaussian form factors and therefore real $\gamma^X_{\mathbf{q}}$. A general expression relating the memory functions $S^{\nu_{\ell'}\mu_{\ell'}}_{\nu_\ell\mu_\ell}$ to the couplings $\gamma^\nu_{\mathbf{q}}$ is given in Ref. 3. For real couplings it simplifies to:

$$S^{\nu_{\ell'}\mu_{\ell'}}_{\nu_\ell\mu_\ell} = - K_{\nu_{\ell'}\nu_\ell}(t_\ell - t_{\ell'}) - K^*_{\mu_\ell\mu_{\ell'}}(t_\ell - t_{\ell'}) + K^*_{\nu_\ell\mu_{\ell'}}(t_\ell - t_{\ell'}) + K_{\nu_{\ell'}\mu_\ell}(t_\ell - t_{\ell'}) \tag{16}$$

with the memory kernel:

$$K_{\nu_\ell\mu_{\ell'}}(\tau) = 2\int_0^\infty d\omega \frac{J_{\nu_\ell\mu_{\ell'}}(\omega)}{\omega^2}\left[1-\cos(\omega\Delta t)\right]\left[\coth\left(\frac{\hbar\omega}{2k_BT}\right)\cos(\omega\tau) - i\sin(\omega\tau)\right], \qquad \tau > 0 \tag{17a}$$

$$K_{\nu_\ell\mu_\ell}(0) = \int_0^\infty d\omega \frac{J_{\nu_\ell\mu_\ell}(\omega)}{\omega^2}\left[\coth\left(\frac{\hbar\omega}{2k_BT}\right)\big(1-\cos(\omega\Delta t)\big) + i\sin(\omega\Delta t) - i\omega\Delta t\right], \tag{17b}$$

where $J_{\nu\mu}(\omega)$ is the spectral density given by:

$$J_{\nu\mu}(\omega) = \sum_j \gamma^\nu_j \gamma^{\mu *}_j \delta(\omega - \omega_j). \tag{18}$$

As can be seen from these explicit expressions, the dynamics of the $N$-level system depends on the bosons only via the spectral density $J_{\nu\mu}(\omega)$, which therefore captures all relevant information of the boson bath. For a linear dispersion $\omega_{\mathbf{q}} = c_s|\mathbf{q}|$ with sound velocity $c_s$ and Gaussian wave functions for electrons and holes with radii $a_e$ and $a_h$, respectively, one obtains the phonon spectral density:

$$J_{\nu\mu}(\omega) = \frac{\omega^3}{4\pi^2\rho\hbar c_s^5}\left(D_e e^{-\omega^2 a_e^2/(4c_s^2)} - D_h e^{-\omega^2 a_h^2/(4c_s^2)}\right)^2 \tag{19}$$

when $\nu, \mu = |X, n\rangle$ and $J_{\nu\mu}(\omega) = 0$ if $\nu = |G, n\rangle$ or $\mu = |G, n\rangle$.

For the calculations in the main article, we use typical values for GaAs-based self-assembled quantum dots [9]: $D_e = 7.0$ eV, $D_h = -3.5$ eV, $\rho = 5370$ kg/m$^3$, $c_s = 5110$ m/s, $a_e/a_h = 1.15$, and $a_e = 3.0$ nm.

## POLARON MASTER EQUATION

In this section we briefly summarize the polaron master equations (PME), the results of which are compared in the main text with the numerically complete path-integral calculations. The PME are a widely used [10–12] approximate approach for the calculation of the dynamics of quantum dots coupled to LA phonons. For more details on this method we refer the reader to the review by Nazir and McCutcheon in Ref. 10.

A standard tool for studying the dynamnics in open quantum systems, i.e., systems of interest coupled to an environment, is the perturbative description using master equations [10] based on the Born-Markov approximation. In second order in the system-environment interaction, one typically ends up with Lindblad-type rate equations describing, e.g., the damping of certain processes in the system due to the interaction with the environment. However, in the case of quantum dots coupled to LA phonons, it has been found [13] that the weak-coupling master equations obtained in this way are only valid for a very limited set of parameters, because they do not account for multi-phonon effects and they do not correctly describe the phonon-induced renormalization of the driving or of the dot-cavity coupling. This problem can be partially circumvented by formulating master equations in the polaron frame[13]. In this approach, a unitary transformation is employed that diagonalizes the dot+phonon Hamiltonian in the absence of driving and coupling to a cavity, i.e., it removes the dot-phonon interaction term. Physically, the transformed states can be interpreted as polarons consisting of dot states and a cloud of phonons that follow the evolution of the dot state instantaneously. This picture breaks down when the system is exposed to driving that is strong enough such that the phonons can no longer follow the dynamics of the dot states. Thus, the polaron frame is suitable for many

experimentally realizable situations with weak driving, but can reach its limits for strong driving. Indeed, we have verified that when the PME are applied to the system in the main text in the weak driving limit (not shown) that the results perfectly agree with the path-integral simulations. A further comparison between path-integrals and the PME for driven two-level systems can be found in Ref. 14.

The polaron transformation is established by:

$$H'_N = e^S H_N e^{-S}, \qquad \text{with} \qquad S = |X\rangle\langle X| \sum_{\mathbf{k}} \left(\alpha_{\mathbf{k}} \hat{b}^\dagger_{\mathbf{k}} - \alpha^*_{\mathbf{k}} \hat{b}_{\mathbf{k}}\right), \tag{20}$$

with $\alpha_{\mathbf{k}} = \gamma^X_{\mathbf{k}}/\omega_{\mathbf{k}}$. The Hamiltonian of the dot-cavity system in the polaron frame reads: [12]

$$\hat{H}'_N = \hat{H}'_{\text{sys}} + \hat{H}'_{\text{bath}} + \hat{H}'_{\text{int}}, \tag{21a}$$

$$\text{with} \quad \hat{H}'_{\text{sys}} = \hbar\Delta\omega_{XL}|X'\rangle\langle X'| + \hbar\Delta\omega_{cL}\hat{a}^\dagger\hat{a} + \langle B\rangle\hat{X}_g, \qquad \hat{H}'_{\text{bath}} = \hbar\sum_{\mathbf{k}}\omega_{\mathbf{k}}\hat{b}^\dagger_{\mathbf{k}}\hat{b}_{\mathbf{k}}, \qquad \hat{H}'_{\text{int}} = \hat{X}_g\hat{\zeta}_g + \hat{X}_u\hat{\zeta}_u, \tag{21b}$$

$$\text{and} \quad \hat{B}_\pm = \exp\Big[\pm\sum_{\mathbf{q}}\left(\alpha^*_{\mathbf{q}}\hat{b}_{\mathbf{q}} - \alpha_{\mathbf{q}}\hat{b}^\dagger\right)\Big], \qquad \langle B\rangle = \exp\Big[-\frac{1}{2}\int_0^\infty d\omega\frac{J(\omega)}{\omega^2}\coth\left(\hbar\omega/(2k_BT)\right)\Big], \tag{21c}$$

$$\hat{X}_g = \hbar g\left(\hat{a}^\dagger|0\rangle\langle X'| + |X'\rangle\langle 0|\hat{a}\right) - \hbar f\left(|0\rangle\langle X'| + |X'\rangle\langle 0|\right), \qquad \hat{\zeta}_g = \frac{1}{2}\left(\hat{B}_+ + \hat{B}_- - 2\langle B\rangle\right), \tag{21d}$$

$$\hat{X}_u = -i\hbar g\left(\hat{a}^\dagger|0\rangle\langle X'| - |X'\rangle\langle 0|\hat{a}\right) + i\hbar f\left(|0\rangle\langle X'| - |X'\rangle\langle 0|\right), \qquad \hat{\zeta}_u = \frac{1}{2i}\left(\hat{B}_+ - \hat{B}_-\right). \tag{21e}$$

The Markovian polaron master equations (PME) are established by applying the Born-Markov approximation to the polaron-transformed system coupled to the phonon environment via $\hat{H}'_{\text{int}}$. The resulting equation of motion for the reduced density matrix in the polaron frame $\hat{\rho}'$ reads: [11, 12]:

$$\frac{\partial}{\partial t}\hat{\rho}' = -\frac{i}{\hbar}\left[\hat{H}'_{\text{sys}}, \hat{\rho}'\right] + \kappa\left[\hat{a}\hat{\rho}'\hat{a}^\dagger - \frac{1}{2}\{\hat{\rho}', \hat{a}^\dagger\hat{a}\}_+\right] + \mathcal{K}[\hat{\rho}'], \tag{22}$$

$$\text{with} \qquad \mathcal{K}[\hat{\rho}'] = -\frac{1}{\hbar^2}\Big([\hat{X}_g, \hat{\Phi}_g\hat{\rho}'] + [\hat{X}_u, \hat{\Phi}_u\hat{\rho}'] + \text{H.c.}\Big), \tag{23a}$$

where "H.c." denotes the Hermitian conjugate and

$$\hat{\Phi}_g = \langle B\rangle^2\int_0^\infty d\tau\,\frac{1}{2}\left(e^{\phi(\tau)} + e^{-\phi(\tau)} - 2\right)e^{-\frac{i}{\hbar}\hat{H}'_{\text{sys}}\tau}\hat{X}_g e^{\frac{i}{\hbar}\hat{H}'_{\text{sys}}\tau}, \quad \hat{\Phi}_u = \langle B\rangle^2\int_0^\infty d\tau\,\frac{1}{2}\left(e^{\phi(\tau)} - e^{-\phi(\tau)}\right)e^{-\frac{i}{\hbar}\hat{H}'_{\text{sys}}\tau}\hat{X}_u e^{\frac{i}{\hbar}\hat{H}'_{\text{sys}}\tau}, \tag{23b}$$

with the phonon correlation function:

$$\phi(t) = \int_0^\infty d\omega\frac{J(\omega)}{\omega^2}\left[\coth\left(\hbar\omega/(2k_BT)\right)\cos(\omega t) - i\sin(\omega t)\right]. \tag{23c}$$


[1] N. Makri and D. E. Makarov, The Journal of Chemical Physics **102**, 4600 (1995).
[2] N. Makri and D. E. Makarov, The Journal of Chemical Physics **102**, 4611 (1995).
[3] A. Vagov, M. D. Croitoru, M. Glässl, V. M. Axt, and T. Kuhn, Phys. Rev. B **83**, 094303 (2011).
[4] A. M. Barth, A. Vagov, and V. M. Axt, Phys. Rev. B **94**, 125439 (2016).
[5] H. P. Breuer and F. Petruccione, *The Theory of Open Quantum Systems*, 1st ed. (Oxford University Press, Oxford, 2002).
[6] M. Glässl and V. M. Axt, Phys. Rev. B **86**, 245306 (2012).
[7] A. M. Barth, S. Lüker, A. Vagov, D. E. Reiter, T. Kuhn, and V. M. Axt, Phys. Rev. B **94**, 045306 (2016).
[8] B. Krummheuer, V. M. Axt, and T. Kuhn, Phys. Rev. B **65**, 195313 (2002).
[9] B. Krummheuer, V. M. Axt, T. Kuhn, I. D'Amico, and F. Rossi, Phys. Rev. B **71**, 235329 (2005).
[10] A. Nazir and D. P. S. McCutcheon, Journal of Physics: Condensed Matter **28**, 103002 (2016).
[11] J. Iles-Smith and A. Nazir, Optica **3**, 207 (2016).
[12] C. Roy and S. Hughes, Phys. Rev. X **1**, 021009 (2011).
[13] D. P. S. McCutcheon and A. Nazir, New Journal of Physics **12**, 113042 (2010).
[14] D. P. S. McCutcheon, N. S. Dattani, E. M. Gauger, B. W. Lovett, and A. Nazir, Phys. Rev. B **84**, 081305 (2011).
